# Supplementary material for: Accurate atomic correlation and total energies for correlation consistent effective core potentials
Source: arXiv:1909.12453 ancillary file (2020-02-21)
Supplement: Supplementary file 1 [file supporting.pdf]

# Supporting Information: Accurate atomic correlation and total energies for correlation consistent effective core potentials

Abdulgani Annaberdiyev,[†] Cody A. Melton,[†,‡] M. Chandler Bennett,[†]
Guangming Wang,[†] and Lubos Mitas[†]

†*Department of Physics, North Carolina State University, Raleigh, North Carolina 27695-8202, USA*
‡*Sandia National Laboratories, Albuquerque, New Mexico 87123, USA*

SAND2019-11580 O

## 1 Data in $D_{2h}$ point group

Tables S1, S2, S3, S4, S5, S6, and S7 provide energies in $D_{2h}$ point group for various elements and pseudopotentials. Tables S8, S9, S10, S11, S12, and S13 provide the corresponding kinetic energies in $D_{2h}$ point group.

Table S1: Atomic correlation and total energies [Ha] for the 1st-row elements with ccECPs[He] for indicated basis sets and methods in $D_{2h}$ point group. Post-HF method values correspond to correlation energies. CBS denotes basis set extrapolated values. Values with (*) were not feasible to calculate and represent estimates from the calculated data. aug-cc-pVnZ basis set (cc-pVnZ for Ne).

| Atom | Method | DZ | TZ | QZ | 5Z | 6Z | CBS |
|---|---|---|---|---|---|---|---|
| **H** | ROHF | -0.49999965 | -0.49999965 | -0.49999965 | -0.49999965 | | -0.49999965(1) |
| **He** | CISD | -0.03390801 | -0.03946245 | -0.04103940 | -0.04156934 | -0.04177354 | -0.042065(23) |
| | RHF | -2.86167947 | -2.86167947 | -2.86167948 | -2.86167948 | -2.86167948 | -2.86167948(1) |
| | Total | | | | | | -2.903745(23) |
| **Li** | ROHF | -0.19685279 | -0.19685279 | -0.19685279 | -0.19685279 | | -0.19685279(1) |
| **Be** | CISD | -0.04699395 | -0.04781761 | -0.04806189 | -0.04818173 | -0.04824394 | -0.04834636(12) |
| | RHF | -0.96189258 | -0.96189258 | -0.96189258 | -0.96189259 | -0.96189258 | -0.96189260(2) |
| | Total | | | | | | -1.01023896(12) |
| **B** | CISD | -0.06484682 | -0.07153471 | -0.07300263 | -0.07333752 | -0.07355788 | -0.07369(12) |
| | RCCSD(T) | -0.06593395 | -0.07322628 | -0.07482123 | -0.07518494 | -0.07542931 | -0.07558(13) |
| | UCCSD(T) | -0.06594278 | -0.07327882 | -0.07487428 | -0.07523735 | -0.07548152 | -0.07563(13) |
| | FCI | -0.06633674 | -0.07374227 | -0.07529726 | -0.07564267 | -0.07587512 | -0.07601(13) |
| | ROHF | -2.53929199 | -2.53929951 | -2.53930397 | -2.53930456 | -2.53930597 | -2.539306(1) |
| | Total | | | | | | -2.61531(13) |
| **C** | CISD | -0.07855565 | -0.09409202 | -0.09742648 | -0.09824707 | -0.09879999 | -0.09919(28) |
| | RCCSD(T) | -0.08030708 | -0.09708463 | -0.10069041 | -0.10157747 | -0.10218081 | -0.10261(31) |
| | UCCSD(T) | -0.08034503 | -0.09722437 | -0.10083382 | -0.10172039 | -0.10232381 | -0.10275(31) |
| | CCSDT(Q) | -0.08074613 | -0.09777804 | -0.10134593 | -0.10220841 | -0.10279602 | -0.10320(31) |
| | FCI | -0.08075703 | -0.09778825 | -0.10135573 | -0.10221784 | -0.10280522 | -0.10321(31) |
| | ROHF | -5.31430315 | -5.31431227 | -5.31431802 | -5.31431738 | -5.31431979 | -5.314320(2) |
| | Total | | | | | | -5.41753(31) |
| **N** | CISD | -0.09359382 | -0.11782215 | -0.12363123 | -0.12539949 | -0.12617272 | -0.127077(65) |
| | RCCSD(T) | -0.09564583 | -0.12165286 | -0.12789000 | -0.12977963 | -0.13061050 | -0.131573(76) |
| | UCCSD(T) | -0.09570506 | -0.12185906 | -0.12811222 | -0.12999924 | -0.13083009 | -0.131786(79) |
| | CCSDT(Q) | -0.09598629 | -0.12230085 | -0.12852942 | -0.13038605 | -0.13120254 | -0.132125(84) |
| | FCI | -0.09599171 | -0.12230706 | -0.12853580 | -0.13039205 | -0.131208(*) | -0.132131(85) |
| | ROHF | -9.63386641 | -9.63386651 | -9.63386735 | -9.63386820 | -9.63386789 | -9.6338682(9) |
| | Total | | | | | | -9.765999(85) |
| **O** | CISD | -0.1246492 | -0.1661684 | -0.1782075 | -0.1821435 | -0.1839430 | -0.18621(14) |
| | RCCSD(T) | -0.1285665 | -0.1728490 | -0.1856582 | -0.1897979 | -0.1917074 | -0.19407(18) |
| | UCCSD(T) | -0.1286637 | -0.1730425 | -0.1858716 | -0.1900124 | -0.1919217 | -0.19428(18) |
| | CCSDT(Q) | -0.1289799 | -0.1734730 | -0.1862864 | -0.1903987 | -0.1922914 | -0.19462(18) |
| | FCI | -0.1289761 | -0.1734721 | -0.1862864 | -0.1903(*) | -0.1922(*) | -0.19462(18) |
| | ROHF | -15.6887438 | -15.6896444 | -15.6897753 | -15.6897740 | -15.6897920 | -15.68979(2) |
| | Total | | | | | | -15.88441(18) |
| **F** | CISD | -0.16290810 | -0.21762589 | -0.23569494 | -0.24149765 | -0.24449739 | -0.24799(57) |
| | RCCSD(T) | -0.16862537 | -0.22701406 | -0.24616290 | -0.25226239 | -0.25543329 | -0.25908(63) |
| | UCCSD(T) | -0.16869113 | -0.22713392 | -0.24629766 | -0.25239795 | -0.25556974 | -0.25922(63) |
| | CCSDT(Q) | -0.16895239 | -0.22745581 | -0.24660080 | -0.25267684 | -0.2559(*) | -0.25948(65) |
| | FCI | -0.16894606 | -0.22744583 | | | | |
| | ROHF | -23.93700527 | -23.93782831 | -23.93791497 | -23.93791376 | -23.93792456 | -23.937925(9) |
| | Total | | | | | | -24.19741(65) |
| **Ne** | CISD | -0.18025458 | -0.24989860 | -0.29174759 | -0.30201083 | -0.30627967 | -0.30949(91) |
| | RCCSD(T) | -0.18462256 | -0.25961485 | -0.30453033 | -0.31557498 | -0.32014022 | -0.32361(94) |
| | UCCSD(T) | -0.18462256 | -0.25961472 | -0.30453031 | -0.31557497 | -0.32014021 | -0.32361(94) |
| | CCSDT(Q) | -0.18480612 | -0.25973913 | -0.30463859 | -0.31566443 | -0.3202(*) | -0.32368(96) |
| | RHF | -34.70881857 | -34.70881857 | -34.70881857 | -34.70881857 | -34.70881857 | -34.70881857(3) |
| | Total | | | | | | -35.03250(96) |

Table S2: Atomic correlation and total energies [Ha] for selected elements with BFD ECPs in $D_{2h}$ point group. Notations as in table S1. aug-cc-pVnZ basis set.

| Atom | Method | DZ | TZ | QZ | 5Z | 6Z | CBS |
|---|---|---|---|---|---|---|---|
| **C** | CISD | -0.08218682 | -0.09634560 | -0.09937206 | -0.10014903 | -0.10072325 | -0.10116(30) |
| | RCCSD(T) | -0.08412432 | -0.09947264 | -0.10276136 | -0.10359700 | -0.10422630 | -0.10469(34) |
| | UCCSD(T) | -0.08416583 | -0.09961460 | -0.10290812 | -0.10374218 | -0.10437165 | -0.10484(34) |
| | CCSDT(Q) | -0.08460615 | -0.10018697 | -0.10343924 | -0.10424590 | -0.10485861 | -0.10530(34) |
| | FCI | -0.08461818 | -0.10019762 | -0.10344958 | -0.10425580 | -0.10486826 | -0.10531(34) |
| | ROHF | -5.32901824 | -5.32902791 | -5.32903304 | -5.32903242 | -5.32903425 | -5.329034(2) |
| | Total | | | | | | -5.43434(34) |
| **N** | CISD | -0.09671731 | -0.12005299 | -0.12559499 | -0.12724555 | -0.12802543 | -0.12888(13) |
| | RCCSD(T) | -0.09894790 | -0.12402643 | -0.12998438 | -0.13174854 | -0.13258862 | -0.13350(15) |
| | UCCSD(T) | -0.09900824 | -0.12423526 | -0.13020784 | -0.13196952 | -0.13280967 | -0.13371(15) |
| | CCSDT(Q) | -0.09930931 | -0.12469007 | -0.13063388 | -0.13236535 | -0.13319069 | -0.13406(15) |
| | FCI | -0.09931577 | -0.12469623 | -0.13064048 | -0.13237147 | -0.133197(*) | -0.13407(15) |
| | ROHF | -9.66837630 | -9.66837630 | -9.66837630 | -9.66837632 | -9.66837636 | -9.6683764(2) |
| | Total | | | | | | -9.80244(15) |
| **O** | CISD | -0.1316691 | -0.1708663 | -0.1821616 | -0.1859531 | -0.1877270 | -0.19001(14) |
| | RCCSD(T) | -0.1361045 | -0.1779572 | -0.1899846 | -0.1939762 | -0.1958616 | -0.19826(18) |
| | UCCSD(T) | -0.1362079 | -0.1781587 | -0.1902053 | -0.1941977 | -0.1960834 | -0.19849(19) |
| | CCSDT(Q) | -0.1365493 | -0.1786065 | -0.1906330 | -0.1945964 | -0.1964645 | -0.19887(20) |
| | FCI | -0.1365476 | -0.1786048 | -0.1906327 | -0.1945(*) | -0.1964(*) | -0.19887(20) |
| | ROHF | -15.7074522 | -15.7083474 | -15.7084813 | -15.7084799 | -15.7084963 | -15.70850(2) |
| | Total | | | | | | -15.90737(20) |
| **Si** | CISD | -0.06971290 | -0.08096003 | -0.08330143 | -0.08393851 | -0.08431909 | -0.08465(15) |
| | RCCSD(T) | -0.07168674 | -0.08462009 | -0.08737082 | -0.08811695 | -0.08855472 | -0.08894(16) |
| | UCCSD(T) | -0.07172215 | -0.08485851 | -0.08761415 | -0.08835626 | -0.08879496 | -0.08917(17) |
| | CCSDT(Q) | -0.07227756 | -0.08575195 | -0.08844280 | -0.08913078 | -0.08954322 | -0.08987(17) |
| | FCI | -0.07229743 | -0.08577362 | -0.08846507 | -0.08915166 | -0.08956355 | -0.08988(17) |
| | ROHF | -3.67867214 | -3.67867292 | -3.67867531 | -3.67867557 | -3.67867577 | -3.6786758(2) |
| | Total | | | | | | -3.76856(17) |

Table S3: Atomic correlation and total energies [Ha] for the 2nd-row elements with ccECPs[Ne] in $D_{2h}$ point group. Notations as in table S1. aug-cc-pVnZ basis set (cc-pVnZ for Ar).

| Atom | Method | DZ | TZ | QZ | 5Z | 6Z | CBS |
|---|---|---|---|---|---|---|---|
| **Na** | ROHF | -0.18583098 | -0.18615968 | -0.18620499 | -0.18620544 | | -0.1862059(2) |
| | CISD | -0.03375431 | -0.03488593 | -0.03495923 | -0.03498970 | -0.03503476 | -0.035077(30) |
| **Mg** | RHF | -0.78825768 | -0.78835857 | -0.78839186 | -0.78839376 | -0.78839489 | -0.788396(3) |
| | Total | | | | | | -0.823473(30) |
| | CISD | -0.05263400 | -0.05654840 | -0.05751761 | -0.05782447 | -0.05796196 | -0.058130(11) |
| | RCCSD(T) | -0.05372003 | -0.05815196 | -0.05924415 | -0.05959197 | -0.05974726 | -0.059939(11) |
| | UCCSD(T) | -0.05373423 | -0.05822181 | -0.05931393 | -0.05966124 | -0.05981620 | -0.060007(11) |
| **Al** | FCI | -0.05418690 | -0.05874704 | -0.05978600 | -0.06011384 | -0.06025660 | -0.0604328(79) |
| | ROHF | -1.87708853 | -1.87708645 | -1.87709009 | -1.87709039 | -1.87709061 | -1.8770907(3) |
| | Total | | | | | | -1.9375235(79) |
| | CISD | -0.07148347 | -0.08068087 | -0.08287535 | -0.08362689 | -0.08390427 | -0.084320(48) |
| | RCCSD(T) | -0.07354504 | -0.08431777 | -0.08689537 | -0.08776849 | -0.08809207 | -0.088569(52) |
| | UCCSD(T) | -0.07358321 | -0.08455595 | -0.08713604 | -0.08801058 | -0.08833074 | -0.088807(56) |
| **Si** | CCSDT(Q) | -0.07415484 | -0.08544303 | -0.08794586 | -0.08877492 | -0.08906923 | -0.089501(57) |
| | FCI | -0.07417456 | -0.08546440 | -0.08796749 | -0.08879555 | -0.08908922 | -0.089520(57) |
| | ROHF | -3.67255079 | -3.67254920 | -3.67255262 | -3.67255314 | -3.67255323 | -3.6725533(2) |
| | Total | | | | | | -3.762073(57) |
| | CISD | -0.0872674 | -0.1041457 | -0.1081973 | -0.1095219 | -0.1100142 | -0.110706(64) |
| | RCCSD(T) | -0.0899578 | -0.1098976 | -0.1147390 | -0.1162992 | -0.1168722 | -0.117667(76) |
| | UCCSD(T) | -0.0900033 | -0.1102977 | -0.1151428 | -0.1167031 | -0.1172737 | -0.118066(78) |
| **P** | CCSDT(Q) | -0.0905108 | -0.1113014 | -0.1160981 | -0.1175918 | -0.1181241 | -0.118837(74) |
| | FCI | -0.0905450 | -0.1113280 | -0.1161277 | -0.1176(*) | -0.1181(*) | -0.118867(74) |
| | ROHF | -6.3409664 | -6.3409664 | -6.3409664 | -6.3409664 | -6.3409664 | -6.3409664(1) |
| | Total | | | | | | -6.459833(74) |
| | CISD | -0.1150761 | -0.1477062 | -0.1571694 | -0.1601329 | -0.1612589 | -0.162730(83) |
| | RCCSD(T) | -0.1205488 | -0.1583130 | -0.1692069 | -0.1726164 | -0.1738859 | -0.17556(12) |
| | UCCSD(T) | -0.1206256 | -0.1586182 | -0.1695648 | -0.1729798 | -0.1742491 | -0.17592(12) |
| **S** | CCSDT(Q) | -0.1212334 | -0.1596349 | -0.1706112 | -0.1739650 | -0.1751899 | -0.17676(12) |
| | FCI | -0.1212619 | -0.1596680 | -0.1706499 | -0.1740(*) | -0.1752(*) | -0.17680(12) |
| | ROHF | -9.9189935 | -9.9205928 | -9.9206059 | -9.9206283 | -9.9206406 | -9.92065(6) |
| | Total | | | | | | -10.09745(13) |
| | CISD | -0.14305710 | -0.19039965 | -0.20634077 | -0.21129242 | -0.21319510 | -0.21564(11) |
| | RCCSD(T) | -0.15050816 | -0.20538895 | -0.22362070 | -0.22929092 | -0.23142360 | -0.23420(17) |
| | UCCSD(T) | -0.15057103 | -0.20557900 | -0.22386628 | -0.22954346 | -0.23167677 | -0.23444(17) |
| **Cl** | CCSDT(Q) | -0.15113925 | -0.20651142 | -0.22486325 | -0.23049667 | -0.23263(*) | -0.23535(17) |
| | FCI | -0.15115932 | -0.20654307 | | | | |
| | ROHF | -14.68992169 | -14.69129790 | -14.69132557 | -14.69133957 | -14.69134674 | -14.69135(3) |
| | Total | | | | | | -14.92670(18) |
| | CISD | -0.14172846 | -0.22523355 | -0.25200143 | -0.26029839 | -0.26354799 | -0.26766(11) |
| | RCCSD(T) | -0.14635485 | -0.24208710 | -0.27329000 | -0.28294884 | -0.28664854 | -0.29138(21) |
| | UCCSD(T) | -0.14635487 | -0.24208709 | -0.27329003 | -0.28294886 | -0.28664854 | -0.29138(21) |
| **Ar** | CCSDT(Q) | -0.14660047 | -0.24266875 | -0.27404277 | -0.28371164 | -0.28736669 | -0.29204(24) |
| | FCI | -0.14661423 | -0.24268224 | | | | |
| | RHF | -20.77966277 | -20.77966277 | -20.77966277 | -20.77966277 | -20.77966277 | -20.77966277(1) |
| | Total | | | | | | -21.07170(24) |

Table S4: Atomic correlation and total energies [Ha] for the 2nd-row elements with ccECPs[He] in $D_{2h}$ point group. Notations as in table S1. cc-pCVnZ basis set.

| Atom | Method | DZ | TZ | QZ | 5Z | 6Z | CBS |
|---|---|---|---|---|---|---|---|
| **Na** | CISD | -0.18031248 | -0.27172919 | -0.29544389 | -0.30406634 | -0.30788932 | -0.313410(61) |
| | RCCSD(T) | -0.18344571 | -0.28002589 | -0.30494689 | -0.31397705 | -0.31797296 | -0.323729(64) |
| | UCCSD(T) | -0.18344870 | -0.28003157 | -0.30495305 | -0.31398332 | -0.31797928 | -0.323736(64) |
| | CCSDT(Q) | -0.18353692 | -0.28010235 | -0.3050(*) | -0.3141(*) | -0.3181(*) | -0.323818(64) |
| | ROHF | -47.35715946 | -47.35715947 | -47.35715947 | -47.35715948 | -47.35715948 | -47.3571595(1) |
| | Total | | | | | | -47.680977(64) |
| **Mg** | CISD | -0.19418640 | -0.29280864 | -0.32236519 | -0.33189329 | -0.33599570 | -0.34124(12) |
| | RCCSD(T) | -0.20421196 | -0.30991836 | -0.34168720 | -0.35180972 | -0.35613221 | -0.36159(13) |
| | UCCSD(T) | -0.20421197 | -0.30991843 | -0.34168729 | -0.35180982 | -0.35613232 | -0.36159(13) |
| | CCSDT(Q) | -0.20425786 | -0.31002264 | -0.3418(*) | -0.3519(*) | -0.3563(*) | -0.36171(13) |
| | RHF | -62.92742515 | -62.92742515 | -62.92742515 | -62.92742519 | -62.92742527 | -62.9274253(1) |
| | Total | | | | | | -63.28914(13) |
| **Al** | CISD | -0.22003852 | -0.31517598 | -0.34527439 | -0.35635744 | -0.36102686 | -0.36806(35) |
| | RCCSD(T) | -0.23228632 | -0.33518844 | -0.36750815 | -0.37931814 | -0.38427147 | -0.39169(38) |
| | UCCSD(T) | -0.23229708 | -0.33526445 | -0.36759523 | -0.37940692 | -0.38436088 | -0.39178(37) |
| | CCSDT(Q) | -0.23271205 | -0.33579218 | -0.3681(*) | -0.3800(*) | -0.3850(*) | -0.39240(38) |
| | ROHF | -80.99328467 | -80.99334970 | -80.99337935 | -80.99338556 | -80.99338866 | -80.993389(1) |
| | Total | | | | | | -81.38578(38) |
| **Si** | CISD | -0.2380255 | -0.3416443 | -0.3736974 | -0.3850944 | -0.3901563 | -0.3972932(66) |
| | RCCSD(T) | -0.2506875 | -0.3640548 | -0.3986946 | -0.4108863 | -0.4162704 | -0.4238033(46) |
| | UCCSD(T) | -0.2507063 | -0.3642777 | -0.3989388 | -0.4111313 | -0.4165151 | -0.4240436(35) |
| | CCSDT(Q) | -0.2511863 | -0.3650993 | -0.3998(*) | -0.4121(*) | -0.4174(*) | -0.4250000(35) |
| | ROHF | -101.6261452 | -101.6262120 | -101.6262446 | -101.6262531 | -101.6262562 | -101.6262569(5) |
| | Total | | | | | | -102.0512569(35) |
| **P** | CISD | -0.2543832 | -0.3690643 | -0.4034612 | -0.4157952 | -0.4213758 | -0.429233(66) |
| | RCCSD(T) | -0.2660361 | -0.3925322 | -0.4299939 | -0.4432510 | -0.4492035 | -0.457505(72) |
| | UCCSD(T) | -0.2660517 | -0.3928744 | -0.4303578 | -0.4436120 | -0.4495627 | -0.457855(74) |
| | CCSDT(Q) | -0.2664275 | -0.3937591 | -0.4313(*) | -0.4446(*) | -0.4506(*) | -0.458886(74) |
| | ROHF | -125.2587059 | -125.2587059 | -125.2587059 | -125.2587065 | -125.2587061 | -125.2587067(5) |
| | Total | | | | | | -125.717593(74) |
| **S** | CISD | -0.2793964 | -0.4127255 | -0.4528366 | -0.4672435 | -0.4736476 | -0.482768(41) |
| | RCCSD(T) | -0.2930399 | -0.4421691 | -0.4865684 | -0.5022234 | -0.5090885 | -0.518749(61) |
| | UCCSD(T) | -0.2930866 | -0.4424431 | -0.4868980 | -0.5025637 | -0.5094302 | -0.519090(62) |
| | CCSDT(Q) | -0.2934939 | -0.4433127 | -0.4878(*) | -0.5036(*) | -0.5104(*) | -0.520110(62) |
| | ROHF | -151.9174562 | -151.9188863 | -151.9190867 | -151.9191670 | -151.9191789 | -151.91920(1) |
| | Total | | | | | | -152.439305(63) |
| **Cl** | CISD | -0.3055167 | -0.4571395 | -0.5040043 | -0.5206145 | -0.5282382 | -0.53876(25) |
| | RCCSD(T) | -0.3202308 | -0.4909785 | -0.5433977 | -0.5616090 | -0.5698336 | -0.58104(23) |
| | UCCSD(T) | -0.3202703 | -0.4911532 | -0.5436256 | -0.5618489 | -0.5700754 | -0.58129(23) |
| | CCSDT(Q) | -0.3206352 | -0.4919171 | -0.5445(*) | -0.5627(*) | -0.5710(*) | -0.58219(23) |
| | ROHF | -181.6134018 | -181.6146398 | -181.6148291 | -181.6148963 | -181.6149016 | -181.61491(1) |
| | Total | | | | | | -182.19710(23) |
| **Ar** | CISD | -0.3291259 | -0.4983511 | -0.5527181 | -0.5720171 | -0.5808150 | -0.59302(22) |
| | RCCSD(T) | -0.3438517 | -0.5346209 | -0.5956646 | -0.6169443 | -0.6264745 | -0.63957(18) |
| | UCCSD(T) | -0.3438517 | -0.5346209 | -0.5956646 | -0.6169443 | -0.6264745 | -0.63957(18) |
| | CCSDT(Q) | -0.3441534 | -0.5351650 | -0.5963(*) | -0.6176(*) | -0.6271(*) | -0.64022(18) |
| | RHF | -214.8921598 | -214.8921598 | -214.8921599 | -214.8921604 | -214.8921611 | -214.8921612(8) |
| | Total | | | | | | -215.53238(18) |

Table S5: Atomic correlation and total energies [Ha] for the 3rd-row main group elements with ccECPs in $D_{2h}$ point group. Notations as in table S1. aug-cc-pVnZ basis set (cc-pCVnZ for K, Ca).

| Atom | Method | DZ | TZ | QZ | 5Z | 6Z | CBS |
|---|---|---|---|---|---|---|---|
| **K** | CISD | -0.17702362 | -0.25025818 | -0.27680275 | -0.28486555 | -0.28829755 | -0.29235(21) |
| | RCCSD(T) | -0.18450036 | -0.26859548 | -0.29941325 | -0.30862333 | -0.31247228 | -0.31694(21) |
| | UCCSD(T) | -0.18450996 | -0.26860642 | -0.29942606 | -0.30863645 | -0.31248545 | -0.31695(21) |
| | CCSDT(Q) | -0.18489132 | -0.26921595 | -0.30016619 | -0.30939(*) | -0.31325(*) | -0.31772(22) |
| | ROHF | -27.93462232 | -27.93462232 | -27.93462245 | -27.93462245 | -27.93462530 | -27.934626(4) |
| | Total | | | | | | -28.25235(22) |
| **Ca** | CISD | -0.22929612 | -0.29416623 | -0.32310943 | -0.33133840 | -0.33484191 | -0.33854(38) |
| | RCCSD(T) | -0.25051655 | -0.32692010 | -0.36059895 | -0.37009280 | -0.37412840 | -0.37833(46) |
| | UCCSD(T) | -0.25051659 | -0.32692014 | -0.36059897 | -0.37009283 | -0.37412851 | -0.37833(46) |
| | CCSDT(Q) | -0.25129831 | -0.32773983 | -0.36145323 | -0.37096(*) | -0.37501(*) | -0.37924(46) |
| | RHF | -36.34973416 | -36.34973414 | -36.34973418 | -36.34973433 | -36.34973523 | -36.349736(2) |
| | Total | | | | | | -36.72897(46) |
| **Ga** | CISD | -0.0471675 | -0.0520006 | -0.0532955 | -0.0536905 | -0.0538359 | -0.054021(13) |
| | RCCSD(T) | -0.0479409 | -0.0531965 | -0.0545981 | -0.0550295 | -0.0551881 | -0.055393(15) |
| | UCCSD(T) | -0.0479508 | -0.0532523 | -0.0546542 | -0.0550851 | -0.0552434 | -0.055448(15) |
| | FCI | -0.0482426 | -0.0535917 | -0.0549576 | -0.0553676 | -0.0555165 | -0.055702(13) |
| | ROHF | -1.9842101 | -1.9842115 | -1.9842118 | -1.9842123 | -1.9842123 | -1.9842125(7) |
| | Total | | | | | | -2.039915(13) |
| **Ge** | CISD | -0.0618893 | -0.0715539 | -0.0744101 | -0.0751125 | -0.0754253 | -0.075660(82) |
| | RCCSD(T) | -0.0633774 | -0.0743062 | -0.0775083 | -0.0782960 | -0.0786438 | -0.078905(89) |
| | UCCSD(T) | -0.0634057 | -0.0744932 | -0.0776966 | -0.0784819 | -0.0788279 | -0.079086(89) |
| | CCSDT(Q) | -0.0637885 | -0.0751051 | -0.0782488 | -0.0789902 | -0.0793152 | -0.079530(93) |
| | FCI | -0.0638013 | -0.0751173 | -0.0782614 | -0.0790018 | -0.0793264 | -0.079540(94) |
| | ROHF | -3.6649011 | -3.6649018 | -3.6649020 | -3.6649026 | -3.6649029 | -3.664903(1) |
| | Total | | | | | | -3.744443(94) |
| **As** | CISD | -0.07039641 | -0.08714420 | -0.09165502 | -0.09303262 | -0.09360150 | -0.094288(16) |
| | RCCSD(T) | -0.07212776 | -0.09120004 | -0.09632986 | -0.09787671 | -0.09850951 | -0.099262(18) |
| | UCCSD(T) | -0.07215698 | -0.09150397 | -0.09663415 | -0.09817850 | -0.09880856 | -0.099556(17) |
| | CCSDT(Q) | -0.07246222 | -0.09216830 | -0.09725624 | -0.09874078 | -0.09933940 | -0.100017(24) |
| | FCI | -0.07248341 | -0.09218100 | -0.09727123 | -0.09875(*) | -0.09935(*) | -0.100032(24) |
| | ROHF | -6.06587734 | -6.06587663 | -6.06587765 | -6.06587778 | -6.06587820 | -6.0658782(4) |
| | Total | | | | | | -6.165911(24) |
| **Se** | CISD | -0.0930417 | -0.1238735 | -0.1342895 | -0.1372959 | -0.1385311 | -0.139892(82) |
| | RCCSD(T) | -0.0970224 | -0.1316780 | -0.1433240 | -0.1466501 | -0.1480022 | -0.149470(88) |
| | UCCSD(T) | -0.0970916 | -0.1319178 | -0.1436107 | -0.1469376 | -0.1482886 | -0.149746(91) |
| | CCSDT(Q) | -0.0975463 | -0.1326448 | -0.1443623 | -0.1476235 | -0.1489306 | -0.150289(96) |
| | FCI | -0.0975657 | -0.1326644 | -0.1443871 | -0.1476(*) | -0.1489(*) | -0.150314(96) |
| | ROHF | -9.1485604 | -9.1499852 | -9.1500304 | -9.1500502 | -9.1500535 | -9.150058(4) |
| | Total | | | | | | -9.300372(96) |
| **Br** | CISD | -0.1106854 | -0.1539119 | -0.1730843 | -0.1781924 | -0.1802462 | -0.18219(23) |
| | RCCSD(T) | -0.1159228 | -0.1645191 | -0.1859497 | -0.1916067 | -0.1938530 | -0.19594(25) |
| | UCCSD(T) | -0.1159752 | -0.1646545 | -0.1861409 | -0.1918017 | -0.1940475 | -0.19612(25) |
| | CCSDT(Q) | -0.1164057 | -0.1653027 | -0.1868675 | -0.1924770 | -0.1947(*) | -0.19674(30) |
| | FCI | -0.1164173 | -0.1653206 | | | | |
| | ROHF | -13.1201540 | -13.1215071 | -13.1215404 | -13.1215496 | -13.1215514 | -13.1215524(4) |
| | Total | | | | | | -13.31829(30) |
| **Kr** | CISD | -0.13816713 | -0.18591690 | -0.21246190 | -0.21982064 | -0.22280036 | -0.22586(26) |
| | RCCSD(T) | -0.14505536 | -0.19969369 | -0.22916475 | -0.23733449 | -0.24060491 | -0.24398(25) |
| | UCCSD(T) | -0.14505533 | -0.19969370 | -0.22916475 | -0.23733449 | -0.24060491 | -0.24398(25) |
| | CCSDT(Q) | -0.14545281 | -0.20023839 | -0.22975824 | -0.23790612 | -0.24118(*) | -0.24453(27) |
| | FCI | -0.14546095 | | | | | |
| | RHF | -18.22805984 | -18.22806066 | -18.22806022 | -18.22806208 | -18.22806315 | -18.228065(5) |
| | Total | | | | | | -18.47259(27) |

Table S6: Atomic correlation and total energies [Ha] for Sc-Mn elements with ccECPs[Ne] in $D_{2h}$ point group. Notations as in table S1. cc-pCVnZ basis set.

| Atom | Method | DZ | TZ | QZ | 5Z | CBS |
|---|---|---|---|---|---|---|
| **Sc($^2$D)** | CISD | -0.32796256 | -0.36173730 | -0.37396087 | -0.38010997 | -0.38679(76) |
| | RCCSD(T) | -0.36604310 | -0.40497119 | -0.41878760 | -0.42563016 | -0.43308(80) |
| | UCCSD(T) | -0.36618982 | -0.40514523 | -0.41896722 | -0.42581186 | -0.43327(80) |
| | CCSDT(Q) | -0.36765472 | -0.40664250 | -0.42051(*) | -0.42738(*) | -0.43488(80) |
| | ROHF | -46.12178822 | -46.12210462 | -46.12212554 | -46.12213770 | -46.122138(7) |
| | Total | | | | | -46.55702(80) |
| **Ti($^3$F)** | CISD | -0.35705400 | -0.39826616 | -0.41414637 | -0.42185097 | -0.43071(66) |
| | RCCSD(T) | -0.39748548 | -0.44451483 | -0.46238810 | -0.47102902 | -0.48093(75) |
| | UCCSD(T) | -0.39771070 | -0.44479054 | -0.46267417 | -0.47132242 | -0.48123(75) |
| | CCSDT(Q) | -0.39919402 | -0.44627755 | -0.46422(*) | -0.47289(*) | -0.48285(75) |
| | ROHF | -57.60900801 | -57.60962174 | -57.60970089 | -57.60974274 | -57.60974(2) |
| | Total | | | | | -58.09260(75) |
| **V($^4$F)** | CISD | -0.39906122 | -0.44502617 | -0.46612164 | -0.47512813 | -0.48744(41) |
| | RCCSD(T) | -0.44481779 | -0.49730050 | -0.52152631 | -0.53178845 | -0.54594(55) |
| | UCCSD(T) | -0.44524393 | -0.49778253 | -0.52202801 | -0.53229413 | -0.54646(55) |
| | CCSDT(Q) | -0.45243936 | -0.50511842 | -0.52972(*) | -0.54013(*) | -0.55457(58) |
| | ROHF | -70.88650990 | -70.88687052 | -70.88703541 | -70.88707243 | -70.88712(3) |
| | Total | | | | | -71.44169(58) |
| **Cr($^7$S)** | CISD | -0.42723842 | -0.48776726 | -0.51425496 | -0.52577647 | -0.54103(24) |
| | RCCSD(T) | -0.46229170 | -0.53117291 | -0.56131191 | -0.57436463 | -0.59170(32) |
| | UCCSD(T) | -0.46257604 | -0.53151639 | -0.56168036 | -0.57474085 | -0.59209(33) |
| | CCSDT(Q) | -0.46308970 | -0.53189219 | -0.56207(*) | -0.57514(*) | -0.59253(33) |
| | ROHF | -86.04808378 | -86.04855303 | -86.04855377 | -86.04855525 | -86.04856(1) |
| | Total | | | | | -86.64109(33) |
| **Mn($^6$S)** | CISD | -0.4573916 | -0.5221195 | -0.5522082 | -0.5647893 | -0.58237(83) |
| | RCCSD(T) | -0.5044855 | -0.5779711 | -0.6121330 | -0.6263267 | -0.6463(10) |
| | UCCSD(T) | -0.5049472 | -0.5784922 | -0.6126726 | -0.6268722 | -0.6468(10) |
| | CCSDT(Q) | -0.5056657 | -0.5790926 | -0.61330(*) | -0.62752(*) | -0.6475(10) |
| | ROHF | -103.2441380 | -103.2443328 | -103.2443341 | -103.2443426 | -103.244343(6) |
| | Total | | | | | -103.8919(10) |

Table S7: Atomic correlation and total energies [Ha] for Fe-Zn elements with ccECPs[Ne] in $D_{2h}$ point group. Notations as in table S1. cc-pCVnZ basis set.

| Atom | Method | DZ | TZ | QZ | 5Z | CBS |
|---|---|---|---|---|---|---|
| **Fe($^5$D)** | CISD | -0.5107712 | -0.5884189 | -0.6255361 | -0.6415891 | -0.66360(68) |
| | RCCSD(T) | -0.5650689 | -0.6532492 | -0.6957991 | -0.7140405 | -0.73932(94) |
| | UCCSD(T) | -0.5656015 | -0.6538446 | -0.6964242 | -0.7146814 | -0.73998(94) |
| | CCSDT(Q) | -0.5663308 | -0.6543966 | -0.69701(*) | -0.71528(*) | -0.74062(95) |
| | ROHF | -122.6459835 | -122.6471770 | -122.6472877 | -122.6473522 | -122.64735(3) |
| | Total | | | | | -123.38798(95) |
| **Co($^4$F)** | CISD | -0.5556327 | -0.6469961 | -0.6915813 | -0.7110208 | -0.73767(77) |
| | RCCSD(T) | -0.6143580 | -0.7178064 | -0.7690287 | -0.7912020 | -0.8219(11) |
| | UCCSD(T) | -0.6147478 | -0.7182721 | -0.7695305 | -0.7917233 | -0.8225(11) |
| | CCSDT(Q) | -0.6151622 | -0.7184800 | -0.76975(*) | -0.79195(*) | -0.8227(11) |
| | ROHF | -144.3303296 | -144.3311368 | -144.3312251 | -144.3313383 | -144.33134(7) |
| | Total | | | | | -145.1541(11) |
| **Ni($^3$F)** | CISD | -0.6105621 | -0.7149678 | -0.7670986 | -0.7899040 | -0.82131(93) |
| | RCCSD(T) | -0.6790395 | -0.7964704 | -0.8564234 | -0.8825722 | -0.9189(12) |
| | UCCSD(T) | -0.6795169 | -0.7969812 | -0.8569511 | -0.8831101 | -0.9195(12) |
| | CCSDT(Q) | -0.6881642 | -0.8055330 | -0.86614(*) | -0.89258(*) | -0.9295(13) |
| | ROHF | -168.4614917 | -168.4623094 | -168.4624643 | -168.4625601 | -168.46256(4) |
| | Total | | | | | -169.3920(13) |
| **Ni($^3$D)** | CISD | -0.6465397 | -0.7570184 | -0.8126635 | -0.8370597 | -0.87068(99) |
| | RCCSD(T) | -0.7152275 | -0.8404277 | -0.9054240 | -0.9340263 | -0.9737(12) |
| | UCCSD(T) | -0.7153693 | -0.8406070 | -0.9056235 | -0.9342362 | -0.9739(12) |
| | CCSDT(Q) | -0.7150314 | -0.8396556 | -0.90459(*) | -0.93317(*) | -0.9728(12) |
| | ROHF | -168.4190995 | -168.4200141 | -168.4201874 | -168.4202614 | -168.42026(2) |
| | Total | | | | | -169.3931(12) |
| **Cu($^2$S)** | CISD | -0.6998956 | -0.8247607 | -0.8882785 | -0.9164908 | -0.95506(89) |
| | RCCSD(T) | -0.7738402 | -0.9159891 | -0.9900301 | -1.0231374 | -1.06846(99) |
| | UCCSD(T) | -0.7739280 | -0.9160963 | -0.9901465 | -1.0232562 | -1.06859(99) |
| | CCSDT(Q) | -0.7728824 | -0.9141401 | -0.98803(*) | -1.02107(*) | -1.0664(10) |
| | ROHF | -195.3358266 | -195.3373699 | -195.3373989 | -195.3374008 | -195.337402(3) |
| | Total | | | | | -196.4038(10) |
| **Zn($^1$S)** | CISD | -0.7139072 | -0.8425259 | -0.9112300 | -0.9413355 | -0.9836(15) |
| | RCCSD(T) | -0.7892886 | -0.9339068 | -1.0128710 | -1.0475878 | -1.0964(18) |
| | UCCSD(T) | -0.7892884 | -0.9339071 | -1.0128710 | -1.0475878 | -1.0964(18) |
| | CCSDT(Q) | -0.7881588 | -0.93257(*) | -1.01142(*) | -1.04608(*) | -1.0949(18) |
| | RHF | -225.2750460 | -225.2750619 | -225.2750649 | -225.2750650 | -225.2750654(6) |
| | Total | | | | | -226.3699(18) |

Table S8: Atomic kinetic energies [Ha] for the 1st-row elements with ccECPs[He] in $D_{2h}$ point group. aug-cc-pVnZ basis set (cc-pVnZ for Ne).

| Atom | Method | DZ | TZ | QZ | 5Z | 6Z | CBS |
|---|---|---|---|---|---|---|---|
| **H** | ROHF | 0.49895288 | 0.49894527 | 0.49894533 | 0.49894996 | | 0.498954(2) |
| **He** | RHF | 2.84397485 | 2.84397376 | 2.84398211 | 2.84397542 | 2.84397523 | |
| | CISD | 2.85517271 | 2.87995550 | 2.88332835 | 2.88469493 | 2.88512740 | 2.8855(2) |
| **Li** | ROHF | 0.076680627 | 0.07668018 | 0.07668022 | 0.076680181 | | 0.07668014(2) |
| **Be** | RHF | 0.31367034 | 0.31367174 | 0.31367101 | 0.31366632 | 0.31366995 | |
| | CISD | 0.37996620 | 0.39833731 | 0.40046822 | 0.40078321 | 0.40081561 | 0.40084(2) |
| **B** | ROHF | 1.31350447 | 1.31349404 | 1.31355496 | 1.31357391 | 1.31359811 | |
| | CISD | 1.41469876 | 1.42117834 | 1.42228561 | 1.42284300 | 1.42329158 | |
| | FCI | 1.41542556 | 1.42613474 | 1.42741224 | 1.42804175 | 1.42861274 | 1.4292(3) |
| **C** | ROHF | 3.43448649 | 3.43452459 | 3.43461006 | 3.43456695 | 3.43460019 | |
| | CISD | 3.51440134 | 3.54787465 | 3.55363577 | 3.55426728 | 3.55601079 | |
| | FCI | 3.51956182 | 3.55773078 | 3.56349068 | 3.56417396 | 3.56611336 | 3.568(1) |
| **N** | ROHF | 6.82755984 | 6.82752510 | 6.82741059 | 6.82745134 | 6.82750451 | |
| | CISD | 6.86959909 | 6.94167021 | 6.95467252 | 6.95730143 | 6.95942600 | |
| | FCI | 6.88381613 | 6.95493764 | 6.96746463 | 6.97040477 | 6.9725(*) | 6.975(1) |
| **O** | ROHF | 11.86224486 | 11.85196677 | 11.84561055 | 11.84569222 | 11.84522573 | |
| | CISD | 11.84670197 | 11.98037873 | 12.00382205 | 12.01119666 | 12.01588644 | |
| | FCI | 11.87194641 | 11.99673997 | 12.01975665 | 12.0271(*) | 12.0318(*) | 12.037(2) |
| **F** | ROHF | 18.64790112 | 18.64372752 | 18.64085665 | 18.64113790 | 18.64087260 | |
| | CISD | 18.58827042 | 18.78838611 | 18.83067241 | 18.84305889 | 18.85181858 | |
| | FCI | 18.62961103 | 18.80776779 | 18.8501(*) | 18.8625(*) | 18.8713(*) | 18.880(4) |
| **Ne** | RHF | 28.04250304 | 28.04244770 | 28.04247300 | 28.04248372 | 28.04249187 | |
| | CISD | 28.08774862 | 28.22056329 | 28.28945965 | 28.30015252 | 28.30424228 | |
| | FCI | 28.13283740 | 28.25418488 | 28.3232(*) | 28.3339(*) | 28.3380(*) | 28.342(2) |

Table S9: BFD ECPs kinetic energies [Ha] for selected elements in $D_{2h}$ point group. aug-cc-pVnZ basis set.

| Atom | Method | DZ | TZ | QZ | 5Z | 6Z | CBS |
|---|---|---|---|---|---|---|---|
| **C** | ROHF | 3.31084033 | 3.31081800 | 3.31085129 | 3.31086049 | 3.31085102 | |
| | CISD | 3.39905497 | 3.43220003 | 3.43742568 | 3.43812989 | 3.43999849 | |
| | FCI | 3.40615847 | 3.44250862 | 3.44799624 | 3.44879717 | 3.45089891 | 3.453(1) |
| **N** | ROHF | 6.75184307 | 6.75184179 | 6.75186129 | 6.75186395 | 6.75187214 | |
| | CISD | 6.80039239 | 6.87176435 | 6.88452081 | 6.88688084 | 6.88911504 | |
| | FCI | 6.81628005 | 6.88488882 | 6.89760719 | 6.90031892 | 6.902(*) | 6.905(1) |
| **O** | ROHF | 11.62401280 | 11.61416101 | 11.60826238 | 11.60841749 | 11.60784968 | |
| | CISD | 11.61505675 | 11.75126357 | 11.77397008 | 11.78124454 | 11.78598259 | |
| | FCI | 11.64339918 | 11.76677842 | 11.78982922 | 11.797(*) | 11.802(*) | 11.807(1) |
| **Si** | ROHF | 1.29873413 | 1.29867797 | 1.29868159 | 1.29868539 | 1.29868470 | |
| | CISD | 1.36205739 | 1.38173544 | 1.38679032 | 1.38739856 | 1.38826984 | |
| | FCI | 1.36884694 | 1.39511435 | 1.40164651 | 1.40249077 | 1.40355225 | 1.4046(5) |

Table S10: Atomic kinetic energies [Ha] for the 2nd-row elements with ccECPs[Ne] in $D_{2h}$ point group. aug-cc-pVnZ basis set (cc-pVnZ for Ar).

| Atom | Method | DZ | TZ | QZ | 5Z | 6Z | CBS |
|---|---|---|---|---|---|---|---|
| **Na** | ROHF | 0.08001484 | 0.07483061 | 0.07499744 | 0.07501148 | | 0.07503(1) |
| **Mg** | RHF | 0.23354968 | 0.23199509 | 0.23154500 | 0.23148284 | 0.23146504 | |
| | CISD | 0.26548027 | 0.26330003 | 0.26350512 | 0.26349267 | 0.26348253 | 0.26347(1) |
| **Al** | ROHF | 0.64171529 | 0.64170120 | 0.64171014 | 0.64171922 | 0.64170997 | |
| | CISD | 0.68754888 | 0.69602892 | 0.69844320 | 0.69924004 | 0.69942606 | |
| | FCI | 0.69123111 | 0.70218436 | 0.70489156 | 0.70584538 | 0.70606455 | 0.7063(1) |
| **Si** | ROHF | 1.32892277 | 1.32890008 | 1.32891100 | 1.32891858 | 1.32891625 | |
| | CISD | 1.38960776 | 1.40891463 | 1.41429056 | 1.41587209 | 1.41625538 | |
| | FCI | 1.39608297 | 1.42180744 | 1.42848778 | 1.43049006 | 1.43096395 | 1.4314(2) |
| **P** | ROHF | 2.35490570 | 2.35488943 | 2.35490586 | 2.35489074 | 2.35490457 | |
| | CISD | 2.42502036 | 2.45836717 | 2.46828346 | 2.47067375 | 2.47122928 | |
| | FCI | 2.43225546 | 2.47652736 | 2.48959729 | 2.4920(*) | 2.4926(*) | 2.4931(3) |
| **S** | ROHF | 3.70257242 | 3.70352986 | 3.70393876 | 3.70381590 | 3.70368510 | |
| | CISD | 3.78902994 | 3.84752777 | 3.86973265 | 3.87441933 | 3.87554308 | |
| | FCI | 3.80049085 | 3.87453980 | 3.90402772 | 3.9088(*) | 3.9099(*) | 3.9110(6) |
| **Cl** | ROHF | 5.49623725 | 5.49743938 | 5.49769904 | 5.49766709 | 5.49757874 | |
| | CISD | 5.59987572 | 5.68408507 | 5.72011850 | 5.72800838 | 5.72997729 | |
| | FCI | 5.61423106 | 5.72022458 | 5.756(*) | 5.764(*) | 5.766(*) | 5.768(1) |
| **Ar** | RHF | 7.79589481 | 7.79588297 | 7.79588540 | 7.79591613 | 7.79591535 | |
| | CISD | 7.94994979 | 8.04531135 | 8.08362249 | 8.08991031 | 8.09141320 | |
| | FCI | 7.95712773 | 8.09128251 | 8.1298(*) | 8.1361(*) | 8.1376(*) | 8.1392(8) |

Table S11: Atomic kinetic energies [Ha] for the 2nd-row elements with ccECPs[He] in $D_{2h}$ point group. cc-pCVnZ basis set.

| Atom | Method | DZ | TZ | QZ | 5Z | 6Z | CBS |
|---|---|---|---|---|---|---|---|
| **Na** | ROHF | 36.52735270 | 36.52739440 | 36.52743838 | 36.52742986 | 36.52742810 | |
| | CISD | 36.56953299 | 36.71379735 | 36.73737044 | 36.74676260 | 36.75035870 | 36.754(2) |
| **Mg** | RHF | 48.55338625 | 48.55353055 | 48.55339130 | 48.55339266 | 48.55340245 | |
| | CISD | 48.72768236 | 48.76011138 | 48.77236767 | 48.78169464 | 48.78598715 | 48.790(2) |
| **Al** | ROHF | 62.89307590 | 62.89299876 | 62.89294356 | 62.89298886 | 62.89297805 | |
| | CISD | 63.02407762 | 63.11878820 | 63.14126507 | 63.15172340 | 63.15583047 | 63.160(2) |
| **Si** | ROHF | 79.41376232 | 79.41369523 | 79.41366270 | 79.41369795 | 79.41371697 | |
| | CISD | 79.56610219 | 79.67094214 | 79.69821018 | 79.70951510 | 79.71421586 | 79.719(2) |
| **P** | ROHF | 98.34763217 | 98.34753767 | 98.34753933 | 98.34759225 | 98.34755827 | |
| | CISD | 98.51183457 | 98.63625664 | 98.66838143 | 98.68140655 | 98.68736394 | 98.693(3) |
| **S** | ROHF | 119.6120740 | 119.6131095 | 119.6122989 | 119.6115298 | 119.6113622 | |
| | CISD | 119.7898780 | 119.9479402 | 119.9867627 | 120.0017791 | 120.0084628 | 120.015(3) |
| **Cl** | ROHF | 144.0484323 | 144.0498567 | 144.0492331 | 144.0486478 | 144.0484987 | |
| | CISD | 144.2370930 | 144.4315014 | 144.4786957 | 144.4966891 | 144.5051791 | 144.514(4) |
| **Ar** | RHF | 170.8576338 | 170.8574905 | 170.8574457 | 170.8574119 | 170.8575078 | |
| | CISD | 171.0530054 | 171.2817089 | 171.3365004 | 171.3576565 | 171.3683304 | 171.379(5) |

Table S12: Atomic kinetic energies [Ha] for the 3rd-row main group elements with ccECPs in $D_{2h}$ point group. aug-cc-pVnZ basis set (cc-pCVnZ for K, Ca).

| Atom | Method | DZ | TZ | QZ | 5Z | 6Z | CBS |
|---|---|---|---|---|---|---|---|
| **K** | ROHF | 10.47154301 | 10.47158948 | 10.47158031 | 10.47154409 | 10.47159990 | |
| | CISD | 10.67094386 | 10.77344574 | 10.80212489 | 10.80724403 | 10.80933057 | 10.811(1) |
| **Ca** | RHF | 13.43105715 | 13.43103412 | 13.43104385 | 13.43103436 | 13.43105075 | |
| | CISD | 13.68784850 | 13.79155454 | 13.83898979 | 13.84842237 | 13.85206945 | 13.856(2) |
| **Ga** | ROHF | 0.71683325 | 0.71680605 | 0.71680712 | 0.71680407 | 0.71680477 | |
| | CISD | 0.75469694 | 0.76107178 | 0.76307324 | 0.76351746 | 0.76378324 | |
| | FCI | 0.75756166 | 0.76513974 | 0.76717115 | 0.76768958 | 0.76797065 | 0.7683(1) |
| **Ge** | ROHF | 1.37340615 | 1.37337458 | 1.37338602 | 1.37337603 | 1.37337625 | |
| | CISD | 1.41821943 | 1.43057985 | 1.43535297 | 1.43619257 | 1.43670066 | |
| | FCI | 1.42262816 | 1.43893523 | 1.44429303 | 1.44525263 | 1.44580878 | 1.4464(3) |
| **As** | ROHF | 2.29918816 | 2.29920741 | 2.29918168 | 2.29919531 | 2.29918832 | |
| | CISD | 2.33822054 | 2.35625126 | 2.36544329 | 2.36747993 | 2.36837897 | |
| | FCI | 2.34192027 | 2.36650052 | 2.37734101 | 2.37938(*) | 2.38029(*) | 2.3812(5) |
| **Se** | ROHF | 3.28150596 | 3.28155565 | 3.28116835 | 3.28122811 | 3.28129767 | |
| | CISD | 3.32695051 | 3.36649686 | 3.38169330 | 3.38591334 | 3.38765336 | |
| | FCI | 3.33284088 | 3.38208380 | 3.40090599 | 3.40515(*) | 3.40689(*) | 3.4086(9) |
| **Br** | ROHF | 4.60159664 | 4.60264039 | 4.60262443 | 4.60262186 | 4.60267005 | |
| | CISD | 4.64630639 | 4.69963977 | 4.72990473 | 4.73726495 | 4.73992399 | |
| | FCI | 4.65339032 | 4.71876957 | 4.74915(*) | 4.75654(*) | 4.75921(*) | 4.762(1) |
| **Kr** | RHF | 6.15676334 | 6.15659795 | 6.15681251 | 6.15675523 | 6.15681101 | |
| | CISD | 6.21644385 | 6.27728282 | 6.31615384 | 6.32677745 | 6.33038286 | |
| | FCI | 6.22657483 | 6.28751(*) | 6.32644(*) | 6.33708(*) | 6.34069(*) | 6.344(2) |

Table S13: Atomic kinetic energies [Ha] for the 3rd-row transition elements with ccECPs[Ne] in $D_{2h}$ point group. cc-pCVnZ basis set.

| Atom | Method | DZ | TZ | QZ | 5Z | CBS |
|---|---|---|---|---|---|---|
| **Sc($^2$D)** | ROHF | 18.81114626 | 18.79436449 | 18.79539726 | 18.79537922 | |
| | CISD | 19.17213606 | 19.20886255 | 19.23330475 | 19.24085720 | 19.248(4) |
| **Ti($^3$F)** | ROHF | 25.88505438 | 25.86810973 | 25.86652880 | 25.86683389 | |
| | CISD | 26.21249355 | 26.27066920 | 26.28930889 | 26.30143649 | 26.314(6) |
| **V($^4$F)** | ROHF | 34.54480419 | 34.54156108 | 34.54100498 | 34.54149363 | |
| | CISD | 34.94715367 | 34.98856053 | 34.98798625 | 35.00157737 | 35.015(7) |
| **Cr($^7$S)** | ROHF | 46.33993725 | 46.34630254 | 46.34615105 | 46.34601850 | |
| | CISD | 46.72814327 | 46.80257628 | 46.81694513 | 46.83905627 | 46.86(1) |
| **Mn($^6$S)** | ROHF | 57.46801485 | 57.45933930 | 57.45978807 | 57.46063830 | |
| | CISD | 57.81481658 | 57.86338258 | 57.87035748 | 57.89245175 | 57.91(1) |
| **Fe($^5$D)** | ROHF | 71.87180119 | 71.85926014 | 71.85945233 | 71.86030431 | |
| | CISD | 72.25959330 | 72.29039068 | 72.28965036 | 72.31302228 | 72.34(1) |
| **Co($^4$F)** | ROHF | 88.37393133 | 88.36093093 | 88.36227973 | 88.36305363 | |
| | CISD | 88.77845411 | 88.80164715 | 88.79657950 | 88.82218324 | 88.85(1) |
| **Ni($^3$F)** | ROHF | 106.9865837 | 106.9809956 | 106.9815402 | 106.9819113 | |
| | CISD | 107.4348622 | 107.4586822 | 107.4451123 | 107.4711444 | 107.50(1) |
| **Ni($^3$D)** | ROHF | 108.5309936 | 108.5416471 | 108.5394343 | 108.5392200 | |
| | CISD | 109.0852647 | 109.1300528 | 109.1067053 | 109.1307579 | 109.15(1) |
| **Cu($^2$S)** | ROHF | 130.0368644 | 130.0605199 | 130.0557909 | 130.0552440 | |
| | CISD | 130.6059338 | 130.6906066 | 130.6536798 | 130.6786121 | 130.70(1) |
| **Zn($^1$S)** | RHF | 150.1003014 | 150.1018032 | 150.1016129 | 150.1016470 | |
| | CISD | 150.6015595 | 150.5955978 | 150.5631498 | 150.5899657 | 150.62(1) |

## 2 Single-determinant FN-DMC energies

This section provides single-determinant FN-DMC energies for ccECP pseudo-atoms. HF nodes in $D_{2h}$ point group with various basis sets are used. The trial wavefunction also includes $J_{eI}$, $J_{ee}$, $J_{eeI}$ Jastrow factors. Tables S14-S46 give these data for various elements in selected timesteps. Table S47 gives the FN-DMC energy comparisons with the exact energy for selected TMs. Note that these references are *not* state-averaged references.

Table S14: DMC total energies for He atom with different basis sets.

| Timestep | DZ | TZ | QZ | 5Z |
|---|---|---|---|---|
| 0.02 | -2.90368(7) | -2.90368(6) | -2.90372(5) | -2.90359(7) |
| 0.01 | -2.90378(6) | -2.90378(5) | -2.90373(5) | -2.90374(5) |
| 0.005 | -2.90373(5) | -2.90372(4) | -2.90376(6) | -2.90369(5) |
| 0.0025 | -2.90369(5) | -2.90368(5) | -2.90374(5) | -2.90370(7) |
| Extrap. | -2.9037206(2) | -2.90374(4) | -2.90375(4) | -2.90374(4) |

Table S15: DMC total energies for Be atom with different basis sets.

| Timestep | DZ | TZ | QZ |
|---|---|---|---|
| 0.02 | -1.0082(3) | -1.0086(3) | -1.0087(3) |
| 0.01 | -1.0085(3) | -1.0089(3) | -1.0087(3) |
| 0.005 | -1.0087(3) | -1.0085(3) | -1.0084(3) |
| 0.0025 | -1.0089(2) | -1.0084(2) | -1.0084(2) |
| Extrap. | -1.0089(2) | -1.0085(2) | -1.0084(2) |

Table S16: DMC total energies for B atom with different basis sets.

| Timestep | DZ | TZ | QZ | 5Z |
|---|---|---|---|---|
| 0.02 | -2.6049(1) | -2.60496(9) | -2.60531(9) | -2.60446(8) |
| 0.01 | -2.6049(1) | -2.60479(9) | -2.6052(1) | -2.60441(9) |
| 0.005 | -2.6045(1) | -2.6047(1) | -2.6048(1) | -2.60438(9) |
| 0.0025 | -2.6052(1) | -2.60455(9) | -2.60490(9) | -2.60439(8) |
| 0.001 | -2.60464(9) | -2.60449(9) | -2.6049(1) | -2.6043(1) |
| Extrap. | -2.6047(2) | -2.60452(4) | -2.60481(7) | -2.60436(1) |

Table S17: DMC Total energies for C atom with different basis

| Timestep | DZ | TZ | QZ | 5Z | 6Z |
|---|---|---|---|---|---|
| 0.02 | -5.4055(1) | -5.4058(1) | -5.4057(1) | -5.4058(1) | -5.4060(1) |
| 0.01 | -5.4055(1) | -5.4050(1) | -5.4050(1) | -5.4050(1) | -5.4055(1) |
| 0.0075 | -5.4049(1) | -5.4049(1) | -5.4050(1) | -5.4049(1) | -5.4052(1) |
| 0.005 | -5.4050(1) | -5.4050(1) | -5.4048(1) | -5.4047(1) | -5.4050(1) |
| Extrap. | -5.4049(3) | -5.4046(1) | -5.4045(1) | -5.40432(3) | -5.4047(1) |

Table S18: DMC total energies for N atom with different basis sets.

| Timestep | DZ | TZ | QZ | 5Z |
|---|---|---|---|---|
| 0.02 | -9.7535(1) | -9.7543(1) | -9.7541(1) | -9.7539(1) |
| 0.01 | -9.7538(1) | -9.7541(1) | -9.7540(1) | -9.7540(1) |
| 0.005 | -9.7536(1) | -9.7545(1) | -9.7539(1) | -9.7541(1) |
| 0.0025 | -9.7536(1) | -9.7540(1) | -9.7538(1) | -9.7539(1) |
| 0.001 | -9.7536(1) | -9.7540(1) | -9.7538(1) | -9.7538(1) |
| Extrap. | -9.75363(8) | -9.7541(1) | -9.75381(2) | -9.75391(9) |

Table S19: DMC total energies for O atom with different basis sets.

| Timestep | DZ | TZ | QZ | 5Z |
|---|---|---|---|---|
| 0.02 | -15.8702(2) | -15.8730(2) | -15.8698(1) | -15.8708(1) |
| 0.01 | -15.8698(2) | -15.8713(2) | -15.8694(2) | -15.8696(1) |
| 0.005 | -15.8697(1) | -15.8701(2) | -15.8697(1) | -15.8695(1) |
| 0.0025 | -15.8694(1) | -15.8694(2) | -15.8691(1) | -15.8695(1) |
| 0.001 | -15.8695(1) | -15.8695(2) | -15.8689(1) | -15.8690(2) |
| Extrap. | -15.86942(6) | -15.8691(1) | -15.8691(2) | -15.8691(2) |

Table S20: DMC total energies for F atom with different basis sets.

| Timestep | DZ | TZ | QZ |
|---|---|---|---|
| 0.02 | -24.1858(4) | -24.1860(3) | -24.1854(4) |
| 0.01 | -24.1839(3) | -24.1835(3) | -24.1840(2) |
| 0.005 | -24.1825(2) | -24.1828(3) | -24.1830(2) |
| 0.0025 | -24.1820(2) | -24.1823(2) | -24.1821(3) |
| Extrap. | -24.1815(2) | -24.1818(2) | -24.1820(2) |

Table S21: DMC total energies for Ne atom with different basis sets.

| Timestep | DZ | TZ | QZ |
|---|---|---|---|
| 0.02 | -35.0255(4) | -35.0253(4) | -35.0255(5) |
| 0.01 | -35.0232(3) | -35.0227(3) | -35.0232(3) |
| 0.005 | -35.0223(3) | -35.0220(2) | -35.0219(3) |
| 0.0025 | -35.0214(3) | -35.0215(3) | -35.0214(3) |
| Extrap. | -35.0210(2) | -35.0209(2) | -35.0207(2) |

Table S22: DMC total energies for Mg atom with different basis sets.

| Timestep | DZ | TZ | QZ | 5Z |
|---|---|---|---|---|
| 0.02 | -0.82309(3) | -0.82306(3) | -0.82309(3) | -0.82307(3) |
| 0.01 | -0.82296(3) | -0.82308(3) | -0.82306(3) | -0.82306(3) |
| 0.005 | -0.82300(4) | -0.82317(3) | -0.82309(3) | -0.82300(3) |
| 0.0025 | -0.82303(3) | -0.82308(3) | -0.82302(3) | -0.82312(3) |
| 0.001 | -0.82303(3) | -0.82307(3) | -0.82309(3) | -0.82298(3) |
| Extrap. | -0.82300(3) | -0.82310(3) | -0.82306(2) | -0.82302(4) |

Table S23: DMC total energies for Al atom with different basis sets.

| Timestep | DZ | TZ | QZ | 5Z |
|---|---|---|---|---|
| 0.02 | -1.93600(6) | -1.93559(7) | -1.93567(7) | -1.93587(6) |
| 0.01 | -1.93583(6) | -1.93563(6) | -1.93584(7) | -1.93586(6) |
| 0.005 | -1.93612(6) | -1.93558(6) | -1.93562(6) | -1.93584(7) |
| 0.0025 | -1.93587(6) | -1.93553(6) | -1.93570(6) | -1.93588(6) |
| 0.001 | -1.93599(6) | -1.93574(6) | -1.93589(6) | -1.93597(6) |
| Extrap. | -1.93595(9) | -1.93563(6) | -1.93579(9) | -1.93591(3) |

Table S24: DMC total energies for Si atom with different basis sets.

| Timestep | DZ | TZ | QZ | 5Z |
|---|---|---|---|---|
| 0.02 | -3.75897(7) | -3.75934(8) | -3.75895(8) | -3.75918(7) |
| 0.01 | -3.75902(7) | -3.75911(7) | -3.75894(7) | -3.75914(7) |
| 0.005 | -3.75902(8) | -3.75933(8) | -3.75905(8) | -3.75914(8) |
| 0.0025 | -3.75895(8) | -3.75920(7) | -3.75893(8) | -3.75914(8) |
| 0.001 | -3.75907(8) | -3.75913(8) | -3.75876(7) | -3.75914(8) |
| Extrap. | -3.75903(3) | -3.75917(7) | -3.75888(8) | -3.759131(5) |

Table S25: DMC total energies for P atom with different basis sets.

| Timestep | DZ | TZ | QZ | 5Z |
|---|---|---|---|---|
| 0.02 | -6.45627(9) | -6.45611(9) | -6.45609(9) | -6.45641(9) |
| 0.01 | -6.4563(1) | -6.45622(8) | -6.4561(1) | -6.45640(9) |
| 0.005 | -6.45642(9) | -6.45641(9) | -6.45610(8) | -6.45659(9) |
| 0.0025 | -6.45647(9) | -6.4561(1) | -6.45632(9) | -6.4562(1) |
| 0.001 | -6.45647(9) | -6.45629(9) | -6.4562(1) | -6.45656(9) |
| Extrap. | -6.45648(1) | -6.4563(1) | -6.45624(6) | -6.4565(1) |

Table S26: DMC total energies for S atom with different basis sets.

| Timestep | DZ | TZ | QZ | 5Z |
|---|---|---|---|---|
| 0.02 | -10.0905(1) | -10.0904(1) | -10.0901(1) | -10.0901(1) |
| 0.01 | -10.0906(1) | -10.0903(1) | -10.0903(1) | -10.0903(1) |
| 0.005 | -10.0906(1) | -10.0905(1) | -10.0903(1) | -10.0903(1) |
| 0.0025 | -10.0907(1) | -10.0905(1) | -10.0905(1) | -10.0902(1) |
| 0.001 | -10.0907(1) | -10.0904(1) | -10.0905(1) | -10.0901(1) |
| Extrap. | -10.09066(3) | -10.09046(6) | -10.09050(4) | -10.09023(8) |

Table S27: DMC total energies for Cl atom with different basis sets.

| Timestep | DZ | TZ | QZ | 5Z |
|---|---|---|---|---|
| 0.02 | -14.9178(2) | -14.9171(1) | -14.9172(2) | -14.9175(1) |
| 0.01 | -14.9181(1) | -14.9175(1) | -14.9173(2) | -14.9167(1) |
| 0.005 | -14.9179(1) | -14.9175(1) | -14.9173(2) | -14.9172(1) |
| 0.0025 | -14.9176(1) | -14.9175(1) | -14.9176(2) | -14.9173(1) |
| 0.001 | -14.9179(2) | -14.9171(1) | -14.9177(1) | -14.9176(1) |
| Extrap. | -14.9178(1) | -14.9174(2) | -14.91759(7) | -14.9173(3) |

Table S28: DMC total energies for Ar atom with different basis sets.

| Timestep | DZ | TZ | QZ | 5Z |
|---|---|---|---|---|
| 0.02 | -21.0615(2) | -21.0617(2) | -21.0614(2) | -21.0615(2) |
| 0.01 | -21.0613(2) | -21.0615(2) | -21.0616(1) | -21.0616(2) |
| 0.005 | -21.0615(2) | -21.0616(2) | -21.0615(2) | -21.0618(2) |
| 0.0025 | -21.0615(2) | -21.0615(2) | -21.0618(2) | -21.0617(2) |
| 0.001 | -21.0611(2) | -21.0613(2) | -21.0615(2) | -21.0618(2) |
| Extrap. | -21.0613(1) | -21.06141(7) | -21.0617(1) | -21.06177(5) |

Table S29: DMC total energies for K atom with different basis sets.

| Timestep | DZ | TZ | QZ |
|---|---|---|---|
| 0.02 | -28.2401(3) | -28.2398(4) | -28.2398(4) |
| 0.01 | -28.2395(3) | -28.2399(3) | -28.2397(3) |
| 0.005 | -28.2395(3) | -28.2394(3) | -28.2392(3) |
| 0.0025 | -28.2393(2) | -28.2393(2) | -28.2395(2) |
| Extrap. | -28.2393(2) | -28.2393(2) | -28.2393(2) |

Table S30: DMC total energies for Ca atom with different basis sets.

| Timestep | DZ | TZ | QZ |
|---|---|---|---|
| 0.02 | -36.7069(4) | -36.7069(6) | -36.7058(5) |
| 0.01 | -36.7057(4) | -36.7054(3) | -36.7058(4) |
| 0.005 | -36.7049(4) | -36.7056(3) | -36.7057(3) |
| 0.0025 | -36.7056(4) | -36.7049(3) | -36.7051(3) |
| Extrap. | -36.7047(3) | -36.7049(3) | -36.7054(2) |

Table S31: DMC total energies for Sc atom with different basis sets.

| Timestep | DZ | TZ | QZ | 5Z |
|---|---|---|---|---|
| 0.02 | -46.5227(5) | -46.5238(5) | -46.5228(5) | -46.5232(5) |
| 0.01 | -46.5211(5) | -46.5213(4) | -46.5200(5) | -46.5221(4) |
| 0.005 | -46.5205(5) | -46.5211(5) | -46.5214(4) | -46.5205(5) |
| 0.0025 | -46.5204(5) | -46.5194(5) | -46.5199(5) | -46.5202(4) |
| 0.001 | -46.5190(4) | -46.5201(4) | -46.5193(4) | -46.5197(4) |
| Extrap. | -46.5193(3) | -46.5196(3) | -46.5195(6) | -46.5197(3) |

Table S32: DMC total energies for Ti atom with different basis sets.

| Timestep | DZ | TZ | QZ | 5Z |
|---|---|---|---|---|
| 0.02 | -58.0538(5) | -58.0535(6) | -58.0530(6) | -58.0518(5) |
| 0.01 | -58.0483(5) | -58.0481(6) | -58.0484(6) | -58.0481(5) |
| 0.005 | -58.0461(5) | -58.0469(5) | -58.0463(5) | -58.0468(5) |
| 0.0025 | -58.0464(5) | -58.0463(5) | -58.0458(6) | -58.0458(5) |
| 0.001 | -58.0453(4) | -58.0458(5) | -58.0458(5) | -58.0453(6) |
| Extrap. | -58.0446(5) | -58.0451(4) | -58.0448(4) | -58.0450(1) |

Table S33: DMC total energies for V atom with different basis sets.

| Timestep | DZ | TZ | QZ | 5Z |
|---|---|---|---|---|
| 0.02 | -71.3831(5) | -71.3826(6) | -71.3830(7) | -71.3834(6) |
| 0.01 | -71.3780(6) | -71.3780(6) | -71.3781(6) | -71.3785(6) |
| 0.005 | -71.3758(6) | -71.3772(5) | -71.3742(7) | -71.3765(7) |
| 0.0025 | -71.3734(6) | -71.3734(4) | -71.3748(5) | -71.3736(6) |
| 0.001 | -71.3756(4) | -71.3738(4) | -71.3727(6) | -71.3741(5) |
| Extrap. | -71.3740(8) | -71.3732(7) | -71.3728(5) | -71.3733(5) |

Table S34: DMC total energies for Cr atom with different basis sets.

| Timestep | DZ | TZ | QZ | 5Z |
|---|---|---|---|---|
| 0.02 | -86.5976(6) | -86.5992(6) | -86.5987(7) | -86.6003(7) |
| 0.01 | -86.5927(6) | -86.5935(5) | -86.5929(6) | -86.5943(6) |
| 0.005 | -86.5893(5) | -86.5900(5) | -86.5900(6) | -86.5914(6) |
| 0.0025 | -86.5857(5) | -86.5890(6) | -86.5885(7) | -86.5874(5) |
| 0.001 | -86.5852(6) | -86.5875(6) | -86.5869(5) | -86.5873(6) |
| Extrap. | -86.5850(7) | -86.5871(2) | -86.5866(2) | -86.5867(7) |

Table S35: DMC total energies for Mn atom with different basis sets.

| Timestep | DZ | TZ | QZ | 5Z |
|---|---|---|---|---|
| 0.02 | -103.8390(7) | -103.8403(7) | -103.8422(7) | -103.8415(8) |
| 0.01 | -103.8336(6) | -103.8335(7) | -103.8340(7) | -103.8330(8) |
| 0.005 | -103.8301(7) | -103.8314(6) | -103.8290(6) | -103.8296(5) |
| 0.0025 | -103.8287(7) | -103.8259(6) | -103.8282(6) | -103.8264(6) |
| 0.001 | -103.8257(6) | -103.8251(5) | -103.8254(6) | -103.8250(5) |
| Extrap. | -103.8263(7) | -103.825(1) | -103.8251(5) | -103.8246(4) |

Table S36: DMC total energies for Fe atom with different basis sets.

| Timestep | DZ | TZ | QZ | 5Z |
|---|---|---|---|---|
| 0.02 | -123.3241(8) | -123.3298(7) | -123.3294(8) | -123.3289(7) |
| 0.01 | -123.3181(7) | -123.3199(6) | -123.3196(7) | -123.3188(7) |
| 0.005 | -123.3146(6) | -123.3143(6) | -123.3140(7) | -123.3152(6) |
| 0.0025 | -123.3118(5) | -123.3118(7) | -123.3109(8) | -123.3118(7) |
| 0.001 | -123.3102(6) | -123.3106(7) | -123.3099(7) | -123.3105(7) |
| Extrap. | -123.3102(5) | -123.3094(2) | -123.3087(2) | -123.3098(4) |

Table S37: DMC total energies for Co atom with different basis sets.

| Timestep | DZ | TZ | QZ | 5Z |
|---|---|---|---|---|
| 0.02 | -145.0906(7) | -145.0913(8) | -145.0923(8) | -145.0933(9) |
| 0.01 | -145.0791(7) | -145.0810(8) | -145.0808(7) | -145.0799(7) |
| 0.005 | -145.0758(7) | -145.0758(8) | -145.0759(7) | -145.0746(7) |
| 0.0025 | -145.0720(7) | -145.0717(6) | -145.0736(7) | -145.0714(6) |
| 0.001 | -145.0703(8) | -145.0699(5) | -145.0702(7) | -145.0731(6) |
| Extrap. | -145.0695(5) | -145.0691(4) | -145.0700(5) | -145.070(1) |

Table S38: DMC total energies for Ni ($^3F$) atom with different basis sets.

| Timestep | DZ | TZ | QZ | 5Z |
|---|---|---|---|---|
| 0.02 | -169.3132(8) | -169.313(1) | -169.3131(8) | -169.3145(6) |
| 0.01 | -169.3014(8) | -169.3002(8) | -169.3024(8) | -169.3006(9) |
| 0.005 | -169.2934(9) | -169.2941(6) | -169.2961(5) | -169.2957(7) |
| 0.0025 | -169.2893(8) | -169.2909(7) | -169.2911(6) | -169.2921(7) |
| 0.001 | -169.2894(7) | -169.2882(7) | -169.2876(6) | -169.2888(8) |
| Extrap. | -169.2874(7) | -169.2874(2) | -169.288(1) | -169.2885(5) |

Table S39: DMC total energies for Cu atom with different basis sets.

| Timestep | DZ | TZ | QZ | 5Z |
|---|---|---|---|---|
| 0.02 | -196.343(1) | -196.3417(7) | -196.3422(9) | -196.3442(8) |
| 0.01 | -196.3287(8) | -196.330(1) | -196.3313(8) | -196.3291(7) |
| 0.005 | -196.3221(8) | -196.3241(7) | -196.3236(7) | -196.3217(8) |
| 0.0025 | -196.3174(9) | -196.3189(8) | -196.3174(7) | -196.3198(9) |
| 0.001 | -196.3149(8) | -196.3165(7) | -196.3173(7) | -196.3188(7) |
| Extrap. | -196.3139(4) | -196.3161(7) | -196.316(1) | -196.3163(8) |

Table S40: DMC total energies for Zn atom with different basis sets.

| Timestep | DZ | TZ | QZ | 5Z |
|---|---|---|---|---|
| 0.02 | -226.3043(8) | -226.3047(9) | -226.3069(7) | -226.3049(9) |
| 0.01 | -226.2893(8) | -226.2894(8) | -226.2890(7) | -226.2892(8) |
| 0.005 | -226.2833(7) | -226.2848(7) | -226.2830(7) | -226.2829(7) |
| 0.0025 | -226.2795(6) | -226.2798(8) | -226.2789(7) | -226.2772(8) |
| 0.001 | -226.2763(6) | -226.2774(8) | -226.2762(7) | -226.2762(7) |
| Extrap. | -226.2756(4) | -226.2765(7) | -226.2746(7) | -226.2743(6) |

Table S41: DMC total energies for Ga atom with different basis sets.

| Timestep | DZ | TZ | QZ | 5Z |
|---|---|---|---|---|
| 0.02 | -2.0390(2) | -2.0387(2) | -2.0386(2) | -2.0386(4) |
| 0.01 | -2.0393(2) | -2.0388(2) | -2.0393(2) | -2.0386(2) |
| 0.005 | -2.0388(2) | -2.0389(2) | -2.0389(2) | -2.0388(2) |
| 0.0025 | -2.0390(2) | -2.0387(2) | -2.0390(2) | -2.0391(2) |
| Extrap. | -2.0389(2) | -2.0388(2) | -2.0392(2) | -2.0390(2) |

Table S42: DMC total energies for Ge atom with different basis sets.

| Timestep | DZ | TZ | QZ | 5Z |
|---|---|---|---|---|
| 0.02 | -3.7418(4) | -3.7414(3) | -3.7420(4) | -3.7424(4) |
| 0.01 | -3.7421(3) | -3.7419(3) | -3.7421(3) | -3.7425(5) |
| 0.005 | -3.7423(3) | -3.7422(3) | -3.7421(3) | -3.7426(3) |
| 0.0025 | -3.7431(4) | -3.7429(3) | -3.7429(3) | -3.7427(2) |
| Extrap. | -3.7429(3) | -3.7429(3) | -3.7426(3) | -3.7427(2) |

Table S43: DMC total energies for As atom with different basis sets.

| Timestep | DZ | TZ | QZ | 5Z |
|---|---|---|---|---|
| 0.02 | -6.1625(2) | -6.1617(2) | -6.1625(3) | -6.1617(2) |
| 0.01 | -6.1630(2) | -6.1625(3) | -6.1627(2) | -6.1628(2) |
| 0.005 | -6.1625(2) | -6.1634(3) | -6.1629(3) | -6.1633(2) |
| 0.0025 | -6.1630(2) | -6.1632(2) | -6.1632(2) | -6.1629(2) |
| Extrap. | -6.1629(2) | -6.1637(2) | -6.1632(2) | -6.1635(2) |

Table S44: DMC total energies for Se atom with different basis sets.

| Timestep | DZ | TZ | QZ | 5Z |
|---|---|---|---|---|
| 0.02 | -9.2964(1) | -9.2966(2) | -9.2964(1) | -9.2965(1) |
| 0.01 | -9.2967(1) | -9.2964(2) | -9.2963(1) | -9.2964(1) |
| 0.005 | -9.2965(1) | -9.2964(2) | -9.2963(1) | -9.2962(1) |
| 0.0025 | -9.2965(1) | -9.2967(2) | -9.2966(1) | -9.2964(1) |
| Extrap. | -9.2966(1) | -9.2965(1) | -9.2965(1) | -9.2963(1) |

Table S45: DMC total energies for Br atom with different basis sets.

| Timestep | DZ | TZ | QZ | 5Z |
|---|---|---|---|---|
| 0.02 | -13.3133(1) | -13.3134(1) | -13.3133(1) | -13.3134(1) |
| 0.01 | -13.3136(1) | -13.3135(1) | -13.3134(1) | -13.3134(1) |
| 0.005 | -13.3136(1) | -13.3134(1) | -13.3133(1) | -13.3133(1) |
| 0.0025 | -13.3137(1) | -13.3133(1) | -13.3133(1) | -13.3134(1) |
| Extrap. | -13.3138(1) | -13.3133(1) | -13.3133(1) | -13.3133(1) |

Table S46: DMC total energies for Kr atom with different basis sets.

| Timestep | DZ | TZ | QZ | 5Z |
|---|---|---|---|---|
| 0.02 | -18.4679(1) | -18.4679(1) | -18.4684(1) | -18.4679(1) |
| 0.01 | -18.4680(1) | -18.4681(1) | -18.4679(1) | -18.4679(1) |
| 0.005 | -18.4681(1) | -18.4678(1) | -18.4678(1) | -18.4678(1) |
| 0.0025 | -18.4678(1) | -18.4678(1) | -18.4678(1) | -18.4679(1) |
| Extrap. | -18.4679(1) | -18.4678(1) | -18.4675(1) | -18.4680(1) |

Table S47: DMC energy comparisons for selected atoms. HF nodes are used obtained at $D_{2h}$ point group. DMC calculations use $\tau = (0.02, 0.01, 0.005, 0.0025)$ $Ha^{-1}$ timestep extrapolation. Here, $\eta = (100\epsilon)/|E_{corr}|$ where $\epsilon$ represents the total DMC error, namely, combined fixed-node and localization biases.

| Atom | State | "Exact"(Ha) | DMC/HF(Ha) | $\epsilon$(mHa) | $\eta$ |
|---|---|---|---|---|---|
| Ti | ($^3$F) | -58.09263(76) | -58.0450(3) | 47.6(8) | 9.8(2) |
| V | ($^4$F) | -71.44178(59) | -71.3730(2) | 68.8(6) | 12.6(1) |
| Co | ($^4$F) | -145.1541(10) | -145.0711(3) | 83(1) | 10.0(1) |
| Ni | ($^3$F) | -169.3912(12) | -169.2894(3) | 102(1) | 11.1(1) |
| Ni | ($^3$D) | -169.3932(12) | -169.3075(3) | 86(1) | 8.8(1) |

## 3 Multi-determinant FN-DMC energies

This section provides multi-determinant fixed-node DMC energies for selected ccECP pseudoatoms. For Be, B, and C we employ two-configuration nodes obtained from CASSCF with $(2s, 2p)$ active space. Tables S48 and S49 give the data for these elements. All trial wavefunctions also include $J_{eI}$, $J_{ee}$, $J_{eeI}$ Jastrow factors.

Table S50 provides energies for CIPSI vs DMC methods. Table S51 provides data for various ECPs as a demonstration of CIPSI convergence.

Table S48: Two-configuration QMC energies for selected atoms. DMC results are from $\tau = (0.02, 0.01, 0.005, 0.0025)$ $\mathrm{Ha}^{-1}$ time step extrapolations. $D$ represents the determinantal part while $J$ represents the Jastrow factor. All values are in Ha.

| Atom | VMC($D$) | VMC($DJ$) | DMC |
|---|---|---|---|
| Be | -1.00789(5) | -1.00881(6) | -1.0100(2) |
| B | -2.5765(2) | -2.6043(2) | -2.6107(4) |
| C | -5.3349(3) | -5.4014(2) | -5.4086(2) |

Table S49: Two-configuration QMC energy comparisons for selected atoms. DMC results are estimated from $\tau = (0.02, 0.01, 0.005, 0.0025)$ $\mathrm{Ha}^{-1}$ time step extrapolations. Here, $\eta = (100\epsilon)/|E_{corr}|$ where $\epsilon$ represents the total DMC error, namely, the combination of fixed-node and localization biases.

| Atom | "Exact"(Ha) | DMC(Ha) | $\epsilon$(mHa) | $\eta$ |
|---|---|---|---|---|
| Be | -1.01023896(12) | -1.0100(2) | 0.2(2) | 0.5(4) |
| B | -2.61531(13) | -2.6107(4) | 4.6(4) | 6.1(6) |
| C | -5.41753(31) | -5.4086(2) | 8.9(4) | 8.6(4) |

Table S50: Comparison of total energies using different methods and basis sets (cc-pVnZ) for F atom with ccECP[He] (data for Fig. 1 in the main paper). HF reference was used for CIPSI expansions. FN-DMC is extrapolated with $\tau = (0.01, 0.005, 0.0025)$ $\mathrm{Ha}^{-1}$ time steps and Jastrow factor was not included.

| Basis | # Dets. | E(var) | E+PT2 | DMC |
|---|---|---|---|---|
| DZ | 1 | -23.93640517 | -24.10991495 | -24.17037(67) |
| | 22 | -23.99389045 | -24.09304827 | -24.16353(49) |
| | 124 | -24.07182532 | -24.08646612 | -24.17512(40) |
| | 1812 | -24.08547306 | -24.08608680 | -24.18061(57) |
| | 10541 | -24.08585222 | -24.08607544 | -24.18098(81) |
| TZ | 1 | -23.93760798 | -24.18780289 | -24.16974(56) |
| | 12 | -23.96499018 | -24.17884623 | -24.16924(52) |
| | 157 | -24.06565653 | -24.16089033 | -24.17463(49) |
| | 1243 | -24.14796428 | -24.15897770 | -24.18726(55) |
| | 18210 | -24.15693387 | -24.15870476 | -24.18935(71) |
| | 150284 | -24.15829091 | -24.15868605 | -24.1920(11) |
| QZ | 1 | -23.93782653 | -24.21082191 | -24.17021(57) |
| | 14 | -23.96321873 | -24.20217212 | -24.16913(60) |
| | 134 | -24.03003434 | -24.18905589 | -24.17045(58) |
| | 1670 | -24.15135399 | -24.18202990 | -24.18686(53) |
| | 11442 | -24.17628321 | -24.18207832 | -24.19397(62) |
| | 118854 | -24.18042552 | -24.18204947 | -24.19491(82) |

## 4 Energies per electron

Figures S1a and S1b plot the total and kinetic energies per electron, respectively, for all considered ccECP pseudoatoms.

Table S51: Comparison of F atom CIPSI energies for ccECP, BFD, and eCEPP.

| ECP | cc-pVDZ | | | cc-pVTZ | | | cc-pVQZ | | |
|---|---|---|---|---|---|---|---|---|---|
| | # Dets. | E(var) | E+PT2 | # Dets. | E(var) | E+PT2 | # Dets. | E(var) | E+PT2 |
| | 1 | -23.936405 | -24.109915 | 1 | -23.937608 | -24.187803 | 1 | -23.937827 | -24.210822 |
| | 2 | -23.946244 | -24.105803 | 4 | -23.945130 | -24.185023 | 4 | -23.943182 | -24.208629 |
| | 6 | -23.964866 | -24.098356 | 9 | -23.960097 | -24.179539 | 7 | -23.952521 | -24.205347 |
| | 22 | -23.993890 | -24.093048 | 24 | -23.979285 | -24.174556 | 17 | -23.966651 | -24.201345 |
| | 64 | -24.037202 | -24.088332 | 67 | -24.017163 | -24.168348 | 42 | -23.988364 | -24.195238 |
| ccECP | 124 | -24.071825 | -24.086466 | 157 | -24.065657 | -24.160890 | 134 | -24.030034 | -24.189056 |
| | 258 | -24.082848 | -24.086302 | 365 | -24.106130 | -24.159095 | 290 | -24.080455 | -24.183395 |
| | 740 | -24.084809 | -24.086124 | 891 | -24.139887 | -24.158960 | 677 | -24.118162 | -24.182366 |
| | 2333 | -24.085572 | -24.086085 | 1911 | -24.151931 | -24.158935 | 1711 | -24.152144 | -24.182035 |
| | 5713 | -24.085851 | -24.086076 | 5955 | -24.155096 | -24.158759 | 4003 | -24.170274 | -24.182173 |
| | 10541 | -24.085852 | -24.086075 | 18210 | -24.156934 | -24.158705 | 11442 | -24.176283 | -24.182080 |
| | | | | 60965 | -24.158055 | -24.158689 | 35369 | -24.178730 | -24.182057 |
| | | | | 150284 | -24.158291 | -24.158686 | 118854 | -24.180426 | -24.182049 |
| | # Dets. | E(var) | E+PT2 | # Dets. | E(var) | E+PT2 | # Dets. | E(var) | E+PT2 |
| | 1 | -23.937011 | -24.118130 | 1 | -23.938216 | -24.193552 | 1 | -23.938435 | -24.215864 |
| | 2 | -23.946891 | -24.113845 | 4 | -23.945720 | -24.190775 | 4 | -23.943793 | -24.213648 |
| | 6 | -23.965582 | -24.106022 | 9 | -23.960740 | -24.185108 | 7 | -23.953154 | -24.210278 |
| | 22 | -23.994678 | -24.100227 | 34 | -23.986017 | -24.178900 | 17 | -23.967306 | -24.206201 |
| | 64 | -24.042137 | -24.094969 | 76 | -24.029355 | -24.171347 | 49 | -23.991227 | -24.199570 |
| | 120 | -24.076899 | -24.093120 | 211 | -24.082860 | -24.165042 | 151 | -24.036669 | -24.192751 |
| BFD | 254 | -24.088733 | -24.092988 | 475 | -24.122166 | -24.163839 | 332 | -24.088804 | -24.187128 |
| | 740 | -24.091308 | -24.092782 | 1087 | -24.149963 | -24.163847 | 708 | -24.124888 | -24.186518 |
| | 2284 | -24.092175 | -24.092727 | 2749 | -24.157719 | -24.163756 | 1780 | -24.157287 | -24.186203 |
| | 5092 | -24.092517 | -24.092715 | 8739 | -24.160487 | -24.163609 | 4136 | -24.174398 | -24.186312 |
| | 12542 | -24.092540 | -24.092714 | 27643 | -24.162203 | -24.163571 | 11745 | -24.180335 | -24.186192 |
| | | | | 83211 | -24.163040 | -24.163558 | 37090 | -24.182827 | -24.186165 |
| | | | | 128164 | -24.163127 | -24.163568 | 125107 | -24.184548 | -24.186150 |
| | # Dets. | E(var) | E+PT2 | # Dets. | E(var) | E+PT2 | # Dets. | E(var) | E+PT2 |
| | 1 | -23.890536 | -24.066367 | 1 | -23.891632 | -24.143132 | 1 | -23.891880 | -24.165073 |
| | 2 | -23.900514 | -24.062016 | 2 | -23.897008 | -24.140836 | 4 | -23.897156 | -24.162914 |
| | 6 | -23.919361 | -24.054200 | 6 | -23.909645 | -24.135776 | 7 | -23.907024 | -24.159381 |
| | 22 | -23.948558 | -24.048792 | 22 | -23.928561 | -24.130915 | 17 | -23.920974 | -24.155464 |
| | 64 | -23.992191 | -24.044018 | 64 | -23.967693 | -24.123849 | 45 | -23.945821 | -24.147785 |
| | 124 | -24.026979 | -24.042118 | 157 | -24.019437 | -24.115852 | 147 | -23.989325 | -24.142023 |
| eCEPP | 258 | -24.038071 | -24.041949 | 385 | -24.061684 | -24.113959 | 329 | -24.040059 | -24.136817 |
| | 741 | -24.040295 | -24.041732 | 887 | -24.094906 | -24.113803 | 731 | -24.075151 | -24.136223 |
| | 2289 | -24.041138 | -24.041683 | 1883 | -24.106590 | -24.113743 | 1843 | -24.107942 | -24.135943 |
| | 5024 | -24.041451 | -24.041673 | 5798 | -24.109813 | -24.113555 | 4108 | -24.124531 | -24.136086 |
| | 11960 | -24.041476 | -24.041672 | 17774 | -24.111672 | -24.113496 | 11594 | -24.130282 | -24.135972 |
| | | | | 59281 | -24.112818 | -24.113480 | 36461 | -24.132667 | -24.135942 |
| | | | | 132983 | -24.113073 | -24.113490 | 123611 | -24.134347 | -24.135940 |

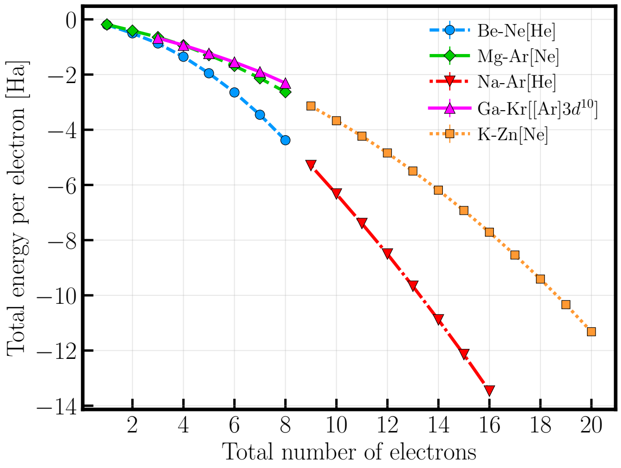


(a) Total energies per electron for ccECPs.

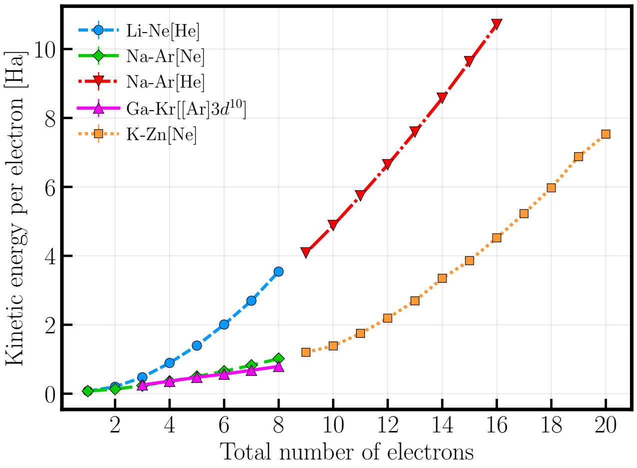


(b) Kinetic energies per electron for ccECPs.

Figure S1
